# Supplementary material for: Establishing Baselines for Photonic Quantum Machine Learning: Insights from an Open, Collaborative Initiative
Source: arXiv:2510.25839 source file (2025-10-29)
Supplement: Supplementary file 1 [file supp_old.tex]

We defined a slightly modified version of the Kronecker Delta to simplify the calculations for different arrangements of the Beam Splitters in our kernel circuits. We use the 0-indexed notation everywhere including indexing the modes and the rows and columns of the matrices. This new BS-delta ($\delta'_{jk}$) is $1$ if the wires indexed $j$ and $k$ are interacting through a BS. This delta can be defined as:
\begin{equation}
    \delta'_{jk} =
    \begin{cases}
        1 & \text{if } j\neq k\ \text{and}\ BS\ \text{present between wires $j$ and $k$} \\
        0 & \text{else}
    \end{cases}
\end{equation}

The matrix for a single layer of Beam Splitters (BS) for a circuit with $m$ modes can be represented as:

\begin{align} \label{eq:sup}
   \begin{bmatrix}
1 & \delta'_{01}\mathrm{i} & \delta'_{02}\mathrm{i} & \cdots & \delta'_{0(m-1)}\mathrm{i} \\
       \delta'_{10}\mathrm{i} & 1 & \cdots & \cdots & \delta'_{1(m-1)}\mathrm{i} \\
       \delta'_{20}\mathrm{i} & \cdots & 1 & \cdots & \delta'_{2(m-1)}\mathrm{i} \\
        \vdots & \vdots & \vdots & \ddots & \vdots \\
        \delta'_{(m-1)0}\mathrm{i} & \cdots & \cdots & \cdots & 1
    \end{bmatrix}
    &= \mathbb{I}_{m\times m} + 
    \begin{bmatrix}
        \delta'_{00}\mathrm{i}^{\delta'_{00}} & \delta'_{01}\mathrm{i} & \cdots & \delta'_{0(m-1)}\mathrm{i} \\
        \delta'_{10}\mathrm{i} & \delta'_{11}\mathrm{i} & \cdots & \delta'_{1(m-1)}\mathrm{i} \\
        \vdots & \vdots & \ddots & \vdots \\
        \delta'_{(m-1)0}\mathrm{i} & \delta'_{(m-1)1}\mathrm{i} & \cdots & \delta'_{(m-1)(m-1)}\mathrm{i}
    \end{bmatrix} \nonumber \\
    &= \mathbb{I}_{m\times m} + 
    \begin{bmatrix}
        0 & \delta'_{01}\mathrm{i} & \cdots & \delta'_{0(m-1)}\mathrm{i} \\
        \delta'_{10}\mathrm{i} & 0 & \cdots & \delta'_{1(m-1)}\mathrm{i} \\
        \vdots & \vdots & \ddots & \vdots \\
        \delta'_{(m-1)0}\mathrm{i} & \delta'_{(m-1)1}\mathrm{i} & \cdots & 0
    \end{bmatrix}
\end{align}


with $j$ being the index of the rows and $k$ the index of the columns of the matrix. $i$ represents the complex number iota. This comes from the matrix for the default BS used by Perceval. Equation~\ref{eq:sup} is unitary due to the fundamental nature of beam splitter operations, which are lossless and energy-preserving. As an example, the matrix for the first and second layers of interference in a $3\times3$ Type~1 kernel circuit, such as in~\ref{fig:type1_circuit}, can be expressed, respectively, as:

\begin{equation}
    M_{L1} = 
    \begin{bmatrix}
        1 & i & 0 & 0 & 0 & 0 & 0 & 0 & 0 \\
        i & 1 & 0 & 0 & 0 & 0 & 0 & 0 & 0 \\
        0 & 0 & 1 & i & 0 & 0 & 0 & 0 & 0 \\
        0 & 0 & i & 1 & 0 & 0 & 0 & 0 & 0 \\
        0 & 0 & 0 & 0 & 1 & i & 0 & 0 & 0 \\
        0 & 0 & 0 & 0 & i & 1 & 0 & 0 & 0 \\
        0 & 0 & 0 & 0 & 0 & 0 & 1 & i & 0 \\
        0 & 0 & 0 & 0 & 0 & 0 & i & 1 & 0 \\
        0 & 0 & 0 & 0 & 0 & 0 & 0 & 0 & 1 \\
    \end{bmatrix}_{9\times9}
    \quad
    M_{L2} = 
    \begin{bmatrix}
        1 & 0 & 0 & 0 & 0 & 0 & 0 & 0 & 0 \\
        0 & 1 & i & 0 & 0 & 0 & 0 & 0 & 0 \\
        0 & i & 1 & 0 & 0 & 0 & 0 & 0 & 0 \\
        0 & 0 & 0 & 1 & i & 0 & 0 & 0 & 0 \\
        0 & 0 & 0 & i & 1 & 0 & 0 & 0 & 0 \\
        0 & 0 & 0 & 0 & 0 & 1 & i & 0 & 0 \\
        0 & 0 & 0 & 0 & 0 & i & 1 & 0 & 0 \\
        0 & 0 & 0 & 0 & 0 & 0 & 0 & 1 & i \\
        0 & 0 & 0 & 0 & 0 & 0 & 0 & i & 1 \\
    \end{bmatrix}_{9\times9}
\end{equation}

Our supplementary ablation studies targeted the core components of the PQK-enhanced architecture to isolate their impact on classification performance.

In both our Type~1 and Type~2 kernel circuits, we use this brickwall-type design of BSs, multiple times. For such an arrangement, the matrices for layers 1 and 2 can be multiplied as:

\begin{equation}
    a_{xy} = \sum_{n=0}^{m-1} M_{L2}[x, n]\cdot M_{L1}[n, y]\ ;\ x, y: 0 \rightarrow m-1
\end{equation}

where $a_{xy}$ is the element at row $x$ and column $y$ and $M_{L1}[x, n]$ is the element at row $x$ and column $n$ in matrix $M_{L1}$. This can be re-written as:

\begin{equation}
    a_{xy} = \sum_{n=0}^{m-1} (\delta_{xn} + \delta^{2'}_{xn}i)\cdot (\delta_{ny} + \delta^{1'}_{ny}i)
    \label{eq:bs_single_layer}
\end{equation}

Here, $\delta^{1'}$ is the $\delta'$ operator for the first layer of the BS arrangement in the 2-layer bricklayer arrangement. Similarly, $\delta^{2'}$ is the $\delta'$ operator for the second layer.

\begin{equation}
    a_{xy} = \sum_{n=0}^{m-1} (\delta_{xn}\cdot\delta_{ny} + \delta_{xn}\cdot\delta^{1'}_{ny}i + \delta_{ny}\cdot\delta^{2'}_{xn}i - \delta^{2'}_{nx}\cdot\delta^{1'}_{yn})
\end{equation}

% Following the definitions of the Kronecker Delta and BS Delta (defined before), we can say that:
% \begin{equation}
%     \delta_{xn}\cdot\delta'_{ny} = \delta'_{xy}
% \end{equation}
% This is because, the left hand side (LHS) will be $1$ if and only if $\delta_{xn}$ is $1$, when $x$ = $n$ and $\delta'_{ny}$ is $1$, when $n$ $\neq$ $y$ and modes $n$ and $y$ interact through a BS. This can be seen as $x$ $\neq$ $y$ and modes $x$ and $y$ interact through a BS. This becomes $\delta'_{xy}$ on the right hand side.

\begin{equation}
    a_{xy} = \delta_{xy} + \delta_{xx}\cdot\delta^{1'}_{xy}i + \delta_{yy}\cdot\delta^{2'}_{xy}i - \sum_{n=0}^{m-1} (\delta^{2'}_{nx}\cdot\delta^{1'}_{yn})
\end{equation}
\begin{equation}
    a_{xy} = \delta_{xy} + \delta^{1'}_{xy}i + \delta^{2'}_{xy}i - \sum_{n=0}^{m-1} (\delta^{2'}_{nx}\cdot\delta^{1'}_{yn})
\end{equation}

We can expand this equation into a piece-wise definition:

\begin{equation}
    a_{xy} = \delta_{xy} + 
    \underbrace{
    \begin{cases} 
        i & \text{if } \delta^{1'}_{xy}=1 \\ 
        0 & \text{if } \delta^{1'}_{xy}=0 
    \end{cases} 
    + 
    \begin{cases} 
        i & \text{if } \delta^{2'}_{xy}=1 \\ 
        0 & \text{if } \delta^{2'}_{xy}=0 
    \end{cases}}_{\in \{0, i\}}
     - \sum_{n=0}^{m-1} (\delta^{2'}_{nx}\cdot\delta^{1'}_{yn})
    % + \sum_{n=0}^{m-1} 
    % \begin{cases} 
    %     -1 & \text{if } \delta^{2'}_{xn}=1 \text{ and } \delta^{1'}_{ny}=1 \\ 
    %     0 & \text{else} 
    % \end{cases}
\end{equation}

The second and third terms can be reduced to either $0$ or $i$. This is because if $\delta^{1'}_{xy}$ is $1$, then $\delta^{2'}_{xy}$ will be $0$. This comes from the bricklayer arrangement that no two consecutive modes interact through a BS in both the layers. However, there can be a case where both these terms are $0$, when $x$ and $y$ are not consecutive modes or $x$ = $y$. The equation now becomes:

\begin{equation}
    a_{xy} = \delta_{xy} + \delta'_{xy}i - \sum_{n=0}^{m-1} (\delta^{2'}_{nx}\cdot\delta^{1'}_{yn})
\end{equation}

The summation in the third term of the equation can be expanded by considering the inner term. This term is non-zero if both $\delta^{2'}_{nx}$ and $\delta^{1'}_{ny}$ are non-zero. This implies that there are BSs present between modes $x$ and $n$ in the first layer and between $y$ and $n$ in the second layer. If such an $n$ exists, the term becomes $-1$ and is $0$ in all other cases. Expanding on the case when the term is non-zero, it is only possible if the indices $x$, $n$ and $y$ are consecutive modes with $x < n < y$ or $y < n < x$ and $x$ and $y$ are at odd-index and even-index mode respectively. In all other cases, the term is $0$. The equation can be expanded as:

\begin{equation}
    a_{xy} = \delta_{xy} + \delta'_{xy}i
    - \sum_{n=0}^{m-1} 
    \begin{cases} 
        1 & \text{if } \delta^{2'}_{xn}=1 \text{ and } \delta^{1'}_{ny}=1 \\ 
        0 & \text{else}
    \end{cases}
\end{equation}

\begin{equation}
    a_{xy} = \delta_{xy} + \delta'_{xy}i
    - 
    \begin{cases} 
        1 & \text{if } \delta_{(x\%2)(y>x)} \text{ and } \lvert x - y\rvert = 2 \\ 
        0 & \text{else}
    \end{cases}
\end{equation}

We can re-write this element assignment as:

\begin{equation}
    a_{xy} = 
    \begin{cases}
        1 & \text{if } \lvert x - y\rvert = 0 \\
        i & \text{if } \lvert x - y\rvert = 1 \\
        -\delta_{(x\%2)(y>x)} & \text{if } \lvert x - y\rvert = 2 \\
        0 & \text{else}
    \end{cases}
    \label{eq:bs_brick}
\end{equation}

% On expanding the summation, the equation can be expanded as:

% \begin{equation}
%     a_{xy} = \delta_{xy} + \delta'_{xy}i
%     - 
%     \begin{cases} 
%         1 & \text{if } \lvert x - y\rvert = 2 \\ 
%         0 & \text{else }
%     \end{cases}
%     \ ;\ x, y: 0 \rightarrow m-1
% \end{equation}

Following this equation, we can form the matrix for a $9$-mode Type~1 kernel (figure~\ref{fig:type1_circuit}) as:

\begin{equation}
    M_{L21} = 
    \begin{bmatrix}
        1 & i & 0 & 0 & 0 & 0 & 0 & 0 & 0 \\
        i & 1 & i & -1 & 0 & 0 & 0 & 0 & 0 \\
        -1 & i & 1 & i & 0 & 0 & 0 & 0 & 0 \\
        0 & 0 & i & 1 & i & -1 & 0 & 0 & 0 \\
        0 & 0 & -1 & i & 1 & i & 0 & 0 & 0 \\
        0 & 0 & 0 & 0 & i & 1 & i & -1 & 0 \\
        0 & 0 & 0 & 0 & -1 & i & 1 & i & 0 \\
        0 & 0 & 0 & 0 & 0 & 0 & i & 1 & i \\
        0 & 0 & 0 & 0 & 0 & 0 & -1 & i & 1
    \end{bmatrix}_{9\times9}
\end{equation}

It can be confirmed that the matrix $M_{l1l2}$ is equal to the matrix obtained after multiplying the matrices $M_{L2}$ and $M_{L1}$. The element assignment rules from equations~\ref{eq:bs_single_layer} and~\ref{eq:bs_brick}, help us in doing the calculations for both types of kernel circuits.

The matrices for patch encoding and assignment of trainable parameters done using Phase Shifters (PS) can be written as:

\begin{equation}
    U_{enc} = 
    \begin{bmatrix}
        e^{ip_0} & 0 & \dots & 0 \\
        0 & e^{ip_1} & \dots & 0 \\
        0 & 0 & \dots & 0 \\
        0 & 0 & \dots & e^{ip_{m-1}}
    \end{bmatrix}_{m\times m}
    \quad
    U_{trainable} = 
    \begin{bmatrix}
        e^{i\theta_0} & 0 & \dots & 0 \\
        0 & e^{i\theta_1} & \dots & 0 \\
        0 & 0 & \dots & 0 \\
        0 & 0 & \dots & e^{i\theta_{m-1}}
    \end{bmatrix}_{m\times m}
\end{equation}

% \begin{equation}
%     a_{xy} = \sum_{n=0}^{8} \delta'_{xn}\cdot\delta'_{ny}\cdot i^{\delta'_{xn}}\cdot i^{\delta'_{ny}}
%            = \sum_{n=0}^{8} \delta'_{xy}\cdot i^{\delta'_{xn}+\delta'_{ny}}
% \end{equation}

% Here, $x$ and $y$ are either equal or unequal. In that case, $\delta'_{xy}$ and $\delta_{xy}$ will be $0$ respectively. Therefore the term becomes:

% \begin{equation}
%     a_{xy} = 9\delta_{xy} + \delta'_{xy}\sum_{n=0}^{8} (i^{\delta'_{xn}+\delta'_{ny}})
% \end{equation}

% The full diagonal phase-shifting operation applied to the \(m \) modes can then be written as the product of patch-encoding and trainable parameter matrices:

% \begin{equation}
%     U_{\phi} = U_{enc} \cdot U_{trainable} = 
%     \begin{bmatrix}
%         e^{i(p_0 + \theta_0)} & 0 & \dots & 0 \\
%         0 & e^{i(p_1 + \theta_1)} & \dots & 0 \\
%         0 & 0 & \dots & 0 \\
%         0 & 0 & \dots & e^{i(p_{m-1} +\theta_{m-1})}
%     \end{bmatrix}_{m\times m}
% \end{equation}
